# Supplementary material for: A Quantitative Understanding of Pattern Matching
Source: arXiv:1912.01914 source file (2019-12-04)
Supplement: Supplementary file 1 [file toappendix.tex]

\gettoappendix {relevance-upper}
\gettoappendix {clash-free-upper}
\gettoappendix {i:qsr}
\gettoappendix {i:se}
\gettoappendix {i:seproof}
\gettoappendix {l:tight-spreading}
\gettoappendix {l:M-tight}
\gettoappendix {l:substitution}
\gettoappendix {l:subject-reduction}
\gettoappendix {l:M-typable-tight}
\gettoappendix {l:anti-substitution}
\gettoappendix {l:subject-expansion}
